# Supplementary material for: FLEET: Butterfly Estimation from a Bipartite Graph Stream
Source: arXiv:1812.03398 source file (2019-08-28)
Supplement: Supplementary file 1 [file reprod-appendix.tex]

\section{Reproducibility Supplement}

\noindent {\bf Source Code:} The source code for our experiments can be directly downloaded from the  link specified in \cite{srccode}.
%: \\
%https://drive.google.com/file/d/1PZWoVjP78Zcf8v55VDr8XAk-yuX1XaSP/view?usp=sharing

\subsection{Compiling and Running the Code}
To compile the code, make sure two prerequisite software already be installed on your computer:
\begin{itemize}
	\item Make tools: we use \textbf{CMake} for managing the build process, version $\geq 2.8$. 
 	\item C++ Compiler: g++ or visual studio C++, support C++11 standard.
\end{itemize}

Our code includes the file \textbf{CMakeLists.txt} for program build, please use the following steps to compile and build to generate executable program:
\begin{itemize}
	\item In the source code folder, type ``cmake CMakeLists.txt''. 
	\item Run ``make'', there will generate executable program named ''stream\_bfly''.
	\item Run ``./stream\_bfly [option]'' to start, where option is the algorithm name. For example, use command ``./stream\_bfly Fleet1'' to run the Fleet1 algorithm. Please refer \textbf{main.cpp} for all the algorithm names.
\end{itemize}

\subsection{Parameter Settings}
Our program provides a user-friendly way to interactively input the parameters. After execute the ``stream\_bfly'' command, please check the printed messages to type in the parameters. The parameter $\gamma$ is the sub-sampling probability -- please refer to the paper for the impact of this parameter. A good value for this parameter is 0.75. The parameter $M$ is the reservoir size -- please refer to the experiments section of the paper to get an idea of the ranges of $M$ that lead to good relative errors for the datasets that we have used. \\

\noindent For sequence-based sliding window, there is a parameter called ``power of $\gamma$'', which sets the sampling probability based on the ratio of the memory budget to the window size $M/W$. For example, when $M/W$ is $5\%$, set this parameter to be $28$, as $0.9^{28} \approx 0.05$. Note that this code uses a default value of 0.9 for $\gamma$\\

\subsection{Datasets}
All the datasets can be downloaded from the link: http://konect.cc/. Here are the detailed download links: \\ \\
Movie-lens: http://konect.cc/networks/movielens-10m\_rating/  \\
Edit-frwiki: http://konect.cc/networks/edit-frwiki/ \\
Edit-enwiki: http://konect.cc/networks/edit-enwiki/  \\
Yahoo-song: http://konect.cc/networks/yahoo-song/  \\
Bag-pubmed: http://konect.cc/networks/bag-pubmed/  \\ \\

The format of raw dataset is givens as list of edges, one edge per line. We preprocessed the raw dataset by removing the duplicate edges in the graph, and for each line only keep the first two numbers which are the two vertices connected by the edge. Preprocessing modules are in ``stream.cpp''. This preprocesses the data and outputs an edge stream. Each element in the resulting edge stream is  a pair of integers representing the edge -- the first number is the vertex in the left partition of the bipartite graph, the second number is the vertex in the right partition.

\subsection{Comparison with Other Algorithms}
To compare with the Graph Priority Sampling algorithm (GPS) and the work of Bera and Chakrabarti (BC), we implemented their algorithms. The code can be found in ``GPS.cpp'' and ``BC.cpp''.
